# Supplementary material for: On Elimination Strategies for Bandit Fixed-Confidence Identification
Source: arXiv:2205.10936 source file (2022-10-24)
Supplement: Supplementary file 1 [file appendix_lower_bounds.tex]

%!TEX root = ../paper.tex

\section{Lower bound proofs}
\label{app:lower_bound_proofs}

For any answer $i$, we have $P_i$ sets $\Lambda_p(i)$, such that $\Lambda(i) = \bigcup_p \Lambda_p(i)$. The elimination stopping time is
\begin{align*}
\tau
= \min \left\{ t \in \mathbb{N} \mid \max_i \min_p \max_{s \le t} (L_s(\hat{\mu}_s, \Lambda_p(i)) - \overline{\log}\frac{1}{\delta} - \gamma(s)) \ge 0 \right\}
 .
\end{align*}
This is simply a rewriting of the following description: $\tau$ is the first time $t$ at which there exists an answer $i$ for which for all sets $\Lambda_p(i)$, there was a time $s \le t$ at which the set was eliminated.

Since $\ihat$ is the argmax for $t = \tau$ in the definition of $\tau$ above, we have $\min_p \max_{s \le \tau} (L_s(\hat{\mu}_s, \Lambda_p(\ihat)) - \overline{\log}\frac{1}{\delta} - \gamma(s)) \ge 0$.

Important equality: $L_s(\hat{\mu}_s, \Lambda_p(i)) = L_s(\hat{\mu}_s, \mu) + L_s(\mu, \Lambda_p(i))$.

With probability $1 - \delta'$, for all $s \in \mathbb{N}$, $L_s(\hat{\mu}_s, \mu) \le \overline{\log} \frac{1}{\delta'} + \gamma(s)$. Hence with probability $1 - \delta'$,
\begin{align*}
&\max_i \min_p \max_{s \le \tau} (L_s(\mu, \Lambda_p(i)) - \overline{\log}\frac{1}{\delta} + \overline{\log}\frac{1}{\delta'}) \ge 0 \: ,
\\
\text{i.e. }& \overline{\log}\frac{1}{\delta} - \max_i \min_p \max_{s \le \tau}  L_s(\mu, \Lambda_p(i)) \le \overline{\log}\frac{1}{\delta'} \: .
\end{align*}
Let $\overline{\exp}$ be the inverse of $\overline{\log}$ \todo{$\overline{\log}$ is supposed increasing and smaller than $2\log$}. We have for all $x \in \overline{\log}^{-1}([1, +\infty))$,
\begin{align*}
\mathbb{P}\left( \overline{\log}\frac{1}{\delta} - \max_i \min_p \max_{s \le \tau}  L_s(\mu, \Lambda_p(i)) > x \right) \le 1/\overline{\exp}(x) \: .
\end{align*}
Since we supposed that $\overline{\log} \le 2 \log$, we have $\overline{\exp}(x) \ge \exp(x/2)$.
\begin{align*}
\mathbb{P}\left( \overline{\log}\frac{1}{\delta} - \max_i \min_p \max_{s \le \tau}  L_s(\mu, \Lambda_p(i)) > x \right) \le e^{-x/2} \: .
\end{align*}

We can get a bound in expectation:
\begin{align*}
&\overline{\log} \frac{1}{\delta} - \mathbb{E}[\max_i \min_p \max_{s \le \tau} L_s(\mu, \Lambda_p(i))]
\\
&\le \mathbb{E}[(\overline{\log}\frac{1}{\delta} - \max_i \min_p \max_{s \le \tau} L_s(\mu, \Lambda_p(i)))\mathbb{I}\{\overline{\log}\frac{1}{\delta} - \max_i \min_p \max_{s \le \tau} L_s(\mu, \Lambda_p(i)) \ge 0\}]
\\
&= \int_0^{+\infty} \mathbb{P}(\overline{\log}\frac{1}{\delta} - \max_i \min_p \max_{s \le \tau} L_s(\mu, \Lambda_p(i)) > x) dx
\\
&\le \overline{\exp}(1) + \int_{\overline{\exp}(1)}^{+\infty} e^{-x/2} dx
\\
&\le e^{1/2} + \int_{0}^{+\infty}e^{-x/2} dx = e^{1/2} + 2
\: .
\end{align*}

\todo[inline]{propagate the changes below}

\begin{align*}
\mathbb{E}[\max_i \min_p \max_{s \le \tau} L_s(\mu, \Lambda_p(i))] \ge \log \frac{1}{\delta} - 1 \: .
\end{align*}

By similar computations with the inequality involving $\ihat$,
\begin{align*}
\mathbb{E}[\min_p \max_{s \le \tau} L_s(\mu, \Lambda_p(\ihat))] \ge \log \frac{1}{\delta} - 1 \: .
\end{align*}

For all $i \ne i^\star$, there exists $m$ such that $\mu \in \Lambda_p(i)$. For that $m$, $L_s(\mu, \Lambda_p(i)) \le L_s(\mu, \mu) = 0$ for all $s \in \mathbb{N}$. Hence for $i\ne i^\star$, $\min_p \max_{s \le \tau} L_s(\mu, \Lambda_p(i)) \le 0$.
\begin{align*}
\min_p \max_{s \le \tau} L_s(\mu, \Lambda_p(\ihat))
&= \mathbb{I}\{\ihat = i^\star\}\min_p \max_{s \le \tau} L_s(\mu, \Lambda_p(\ihat)) + \mathbb{I}\{\ihat \ne i^\star\}\min_p \max_{s \le \tau} L_s(\mu, \Lambda_p(\ihat))
\\
&\le \mathbb{I}\{\ihat = i^\star\}\min_p \max_{s \le \tau} L_s(\mu, \Lambda_p(\ihat))
\\
&= \mathbb{I}\{\ihat = i^\star\}\min_p \max_{s \le \tau} L_s(\mu, \Lambda_p(i^\star))
\\
&= \min_p \max_{s \le \tau} L_s(\mu, \Lambda_p(i^\star)) - \mathbb{I}\{\ihat \ne i^\star\}\min_p \max_{s \le \tau} L_s(\mu, \Lambda_p(i^\star))
\\
&\le \min_p \max_{s \le \tau} L_s(\mu, \Lambda_p(i^\star)) + \mathbb{I}\{\ihat \ne i^\star\} \max_{s \le \tau} L_s(\hat{\mu}_s, \mu)
\end{align*}

\paragraph{Bound on the expectation}
We prove $\mathbb{E}[L_\tau(\hat{\mu}_\tau, \mu)] \le \mathbb{E}[\max_{s \le \tau}L_s(\hat{\mu}_s, \mu)] \le 1 + \mathbb{E}[\gamma(\tau)]$. In the computations below, we use that $s \mapsto \gamma(s)$ is non-decreasing.
\begin{align*}
\mathbb{E}[\max_{s \le \tau}L_s(\hat{\mu}_s, \mu) - \gamma(\tau)]
&\le \mathbb{E}[\max\{0, \max_{s \le \tau}L_s(\hat{\mu}_s, \mu) - \gamma(\tau)\}]
\\
&= \int_{x=0}^{+\infty}\mathbb{P}(\max_{s \le \tau}L_s(\hat{\mu}_s, \mu) - \gamma(\tau) > x) dx
\\
&\le \int_{x=0}^{+\infty}\mathbb{P}(\exists t \in \mathbb{N}, L_t(\hat{\mu}_t, \mu) > x + \gamma(t)) dx
\\
&\le \int_{x=0}^{+\infty} e^{- x} d x = 1
\: .
\end{align*}

\paragraph{Bound on the expectation of the truncated LLR}
\begin{align*}
\mathbb{E}[\mathbb{I}\{\ihat \ne i^\star\} \max_{s \le \tau}L_s(\hat{\mu}_s, \mu)]
&\le \sqrt{\mathbb{P}\{\ihat \ne i^\star\} \mathbb{E}[(\max_{s \le \tau}L_s(\hat{\mu}_s, \mu))^2]}
\end{align*}

\begin{align*}
\mathbb{E}[(\max_{s \le \tau}L_s(\hat{\mu}_s, \mu))^2 - 2\gamma(\tau)^2]
&\le \mathbb{E}[\max\{0, (\max_{s \le \tau}L_s(\hat{\mu}_s, \mu))^2 - 2\gamma(\tau)^2\}]
\\
&= \int_{x=0}^{+\infty}\mathbb{P}((\max_{s \le \tau}L_s(\hat{\mu}_s, \mu))^2 - 2\gamma(\tau)^2 > x) dx
\\
&\le \int_{x=0}^{+\infty}\mathbb{P}((\max_{s \le \tau}L_s(\hat{\mu}_s, \mu))^2 > (\gamma(\tau) + \sqrt{x/2})^2) dx
\\
&= \int_{x=0}^{+\infty}\mathbb{P}(\max_{s \le \tau}L_s(\hat{\mu}_s, \mu) > \gamma(\tau) + \sqrt{x/2} ) dx
\\
&\le \int_{x=0}^{+\infty}\mathbb{P}(\exists t \in \mathbb{N}, L_t(\hat{\mu}_t, \mu) > \gamma(t) + \sqrt{x/2}) dx
\\
&\le \int_{x=0}^{+\infty} e^{- \sqrt{x/2}} d x = 4
\: .
\end{align*}

\begin{align*}
\mathbb{E}[\mathbb{I}\{\ihat \ne i^\star\} \max_{s \le \tau}L_s(\hat{\mu}_s, \mu)]
&\le \sqrt{\mathbb{P}\{\ihat \ne i^\star\} (4 + \mathbb{E}[\gamma(\tau)^2])]}
\: .
\end{align*}
Since the algorithm is $\delta$-correct, $\mathbb{P}\{\ihat \ne i^\star\} \le \delta$.

\paragraph{Special case of LLR stopping}

Note: for LLR stopping, $M_i = 1$ for all $i$ and we get
\begin{align*}
\mathbb{E}[\max_i \max_{s \le \tau} L_s(\mu, \Lambda(i))]
&\ge \log \frac{1}{\delta} - 1
\: , &
\mathbb{E}[\max_{s \le \tau} L_s(\mu, \Lambda(\ihat))]
&\ge \log \frac{1}{\delta} - 1
\: .
\end{align*}
And due to the way the algorithm stops, we could go through the same proof but with $\max_{s \le \tau}$ replaced by taking the value at $\tau$ for the answer $\ihat$. That would give
\begin{align*}
\mathbb{E}[L_\tau(\mu, \Lambda(\ihat))]
&\ge \log \frac{1}{\delta} - 1
\: .
\end{align*}

\begin{align*}
L_\tau(\mu, \Lambda(\ihat))
&= \mathbb{I}\{\ihat = i^\star\}L_\tau(\mu, \Lambda(\ihat)) + \mathbb{I}\{\ihat \ne i^\star\}L_\tau(\mu, \Lambda(\ihat))
\\
&\le \mathbb{I}\{\ihat = i^\star\}L_\tau(\mu, \Lambda(\ihat)) + \mathbb{I}\{\ihat \ne i^\star\}L_\tau(\mu, \mu)
\\
&= \mathbb{I}\{\ihat = i^\star\}L_\tau(\mu, \Lambda(\ihat))
\\
&= \mathbb{I}\{\ihat = i^\star\}L_\tau(\mu, \Lambda(i^\star))
\\
&= L_\tau(\mu, \Lambda(i^\star)) - \mathbb{I}\{\ihat \ne i^\star\} L_\tau(\mu, \Lambda(i^\star))
\\
&= L_\tau(\mu, \Lambda(i^\star)) + \mathbb{I}\{\ihat \ne i^\star\} L_\tau(\hat{\mu}_\tau, \mu)
\end{align*}

\subsection{Expectation of the infimum}
\label{sub:expectation_of_the_infimum}

For a set $\Lambda$ and $\varepsilon \ge 0$, let $\Lambda_{[0,\varepsilon], N_t} = \{\lambda \in \Lambda \mid \sum_k N_t^k \KL_k(\theta, \lambda) \le \inf_{\eta \in \Lambda} \sum_k N_t^k \KL_k(\theta, \eta) + \varepsilon\}$. Then since $\Lambda_{[0,\varepsilon], N_t} \subseteq \Lambda$,
\begin{align*}
\inf_{\lambda \in \Lambda} L_t (\theta, \lambda)
&\le \inf_{\lambda \in \Lambda_{[0,\varepsilon], N_t}} L_t (\theta, \lambda)
\\
&= \inf_{\lambda \in \Lambda_{[0, \varepsilon], N_t}}\left(\sum_k N_t^k \KL_k(\theta, \lambda)
	- \sum_{s=1}^t (\KL_{k_s}(\theta, \lambda) - \log \frac{d \mathbb{P}_\theta}{d \mathbb{P}_\lambda}(X_s^{k_s})) \right)
\\
&\le \inf_{\lambda \in \Lambda} \sum_k N_t^k \KL_k(\theta, \lambda) + \varepsilon
	- \sup_{\lambda \in \Lambda_{[0, \varepsilon], N_t}}\left( \sum_{s=1}^t (\KL_{k_s}(\theta, \lambda) - \log \frac{d \mathbb{P}_\theta}{d \mathbb{P}_\lambda}(X_s^{k_s})) \right)
\: ,\\
\mathbb{E}[\inf_{\lambda \in \Lambda} L_t (\theta, \lambda)]
&\le \inf_{\lambda \in \Lambda}\sum_k \mathbb{E}[N_t^k] \KL_k(\theta, \lambda) + \varepsilon
	- \mathbb{E}\left[\sup_{\lambda \in \Lambda_{[0, \varepsilon], N_t}}\left( \sum_{s=1}^t (\KL_{k_s}(\theta, \lambda) - \log \frac{d \mathbb{P}_\theta}{d \mathbb{P}_\lambda}(X_s^{k_s})) \right)\right]
\: .
\end{align*}

For Gaussian distributions,
\begin{align*}
\mathbb{E}\left[\sup_{\lambda \in \Lambda_{[0, \varepsilon], N_t}}\left( \sum_{s=1}^t (\KL_{k_s}(\theta, \lambda) - \log \frac{d \mathbb{P}_\theta}{d \mathbb{P}_\lambda}(X_s^{k_s})) \right)\right]
&= \mathbb{E}\left[\sup_{\lambda \in \Lambda_{[0, \varepsilon], N_t}} \sum_k N_t^k (\hat{\mu}_{t,k} - \mu_k(\theta)) (\mu_k(\lambda) - \mu_k(\theta))\right]
\end{align*}

Our goal now is to show that this expectected supremum is large, which means that the expected infimum LLR is lower than the infimum of the weighted sum of the KL, hence a lower bound on the infimum LLR is stronger than a lower bound on the weighted sum of KLs.

Let's look at the case of fixed design ($N_t$ is deterministic). Let $\KL(t, \Lambda) = \inf_{\lambda \in \Lambda}\sum_k N_t^k \KL_k(\theta, \lambda)$ and let $u_{\lambda, N_t} = \frac{\mu(\lambda) - \mu(\theta)}{\Vert \mu(\lambda) - \mu(\theta)\Vert_{N_t}} = \frac{\mu(\lambda) - \mu(\theta)}{\sqrt{2 \sum_k N_t^k \KL_k(\theta, \lambda)}}$. The vector $u_{\lambda, N_t}$ has norm 1 for all $\lambda$. Finally, let $Z = \sqrt{N_t^k} (\hat{\mu}_{t,k} - \mu_k(\theta))$. $Z$ has law $\mathcal N(0,1)$.
\begin{align*}
&\mathbb{E}\left[\sup_{\lambda \in \Lambda_{[0, \varepsilon], N_t}} \sum_k N_t^k (\hat{\mu}_{t,k} - \mu_k(\theta)) (\mu_k(\lambda) - \mu_k(\theta))\right]
\\
&= \mathbb{E}\left[\sup_{\lambda \in \Lambda_{[0, \varepsilon], N_t}} \sqrt{2 \sum_k N_t^k \KL_k(\theta, \lambda)} Z^\top u_{\lambda, N_t}\right]
\\
&\ge \sqrt{2} \mathbb{E}\left[\sup_{\lambda \in \Lambda_{[0, \varepsilon], N_t}} \sqrt{\KL(t, \Lambda) + \varepsilon \mathbb{I}\{Z^\top u_{\lambda, N_t}\le 0\}} Z^\top u_{\lambda, N_t}\right]
\end{align*}
For $\varepsilon = 0$, using that $N_t$ is not random (hence $\KL(t, \Lambda)$ isn't either) this is
\begin{align*}
\mathbb{E}\left[\sup_{\lambda \in \Lambda_{\{0\}, N_t}} \sqrt{2 \KL(t, \Lambda)} Z^\top u_{\lambda, N_t}\right]
&= \sqrt{2 \KL(t, \Lambda)} \mathbb{E}\left[\sup_{\lambda \in \Lambda_{\{0\}, N_t}} Z^\top u_{\lambda, N_t}\right]
\end{align*}
The value $\mathbb{E}\left[\sup_{\lambda \in \Lambda_{\{0\}, N_t}} Z^\top u_{\lambda, N_t}\right]$ is the Gaussian width of the set $\{u_{\lambda, N_t} \mid \lambda \in \Lambda_{\{0\}, N_t}\}$, which is a subset of the sphere $\{u \mid \Vert u \Vert = 1\}$.

For unstructured best arm identification, this set contains up to $K-1$ points ($K-1$ exactly at the $N_t$ which maximizes $V_t$). The Gaussian width scales as $\sqrt{\log K}$ in that case.
