# Supplementary material for: On Elimination Strategies for Bandit Fixed-Confidence Identification
Source: arXiv:2205.10936 source file (2022-10-24)
Supplement: Supplementary file 2 [file appendix_opt_allocation.tex]

%!TEX root = ../paper.tex

\section{Deleting Pieces}
\label{sec:deleting_pieces}

The main question we answer in this section is ``what happens to the set of optimal allocations when we delete a piece of the alternative?''.

For a set $\Lambda$, let $\Omega(\Lambda) = \argmax_{\omega \in \triangle_K} \inf_{\lambda \in \Lambda} \sum_{k = 1}^K \omega^k \KL_k(\mu, \lambda)$. $\Omega(\Lambda)$ is a convex and closed set for any set $\Lambda$.

\begin{lemma}\label{lem:optimal_alloc_restrict_alternative_subset}
If $\Lambda' \subseteq \Lambda$ and for some $\varepsilon > 0$, $\{\lambda \in \Lambda \mid \exists \omega \in \Omega(\Lambda), \sum_{k = 1}^K \omega^k \KL_k(\mu, \lambda) \le \inf_{\eta \in \Lambda} \sum_{k = 1}^K \omega^k \KL_k(\mu, \eta) + \varepsilon\} \subseteq \Lambda'$, then $\Omega(\Lambda) \subseteq \Omega(\Lambda')$. 
\end{lemma}
\begin{proof}
TODO: we suppose for now that for all $\omega \in \Omega(\Lambda)$ there exists a distribution $q_\omega$ over points in $\Lambda$ which belongs to a Nash equilibrium.

Those $q_\omega$ distributions are also distributions over $\Lambda'$ since they are supported on points in $\{\lambda \in \Lambda \mid \sum_{k = 1}^K \omega^k \KL_k(\mu, \lambda) = \inf_{\eta \in \Lambda} \sum_{k = 1}^K \omega^k \KL_k(\mu, \eta)\}$. Then for any $\omega \in \triangle_K$ and $\omega^* \in \Omega(\Lambda)$ we have 
\begin{align*}
\inf_{\lambda \in \Lambda'} \sum_k \omega^{k} \KL_k(\mu, \lambda)
&\le \mathbb{E}_{\lambda \sim q_{\omega^*}}\sum_k \omega^k \KL_k(\mu, \lambda)
\\
&\stackrel{(a)}{\le} \mathbb{E}_{\lambda \sim q_{\omega^*}}\sum_k \omega^{*k} \KL_k(\mu, \lambda)
\stackrel{(b)}{=} \inf_{\lambda \in \Lambda} \sum_k \omega^{*k} \KL_k(\mu, \lambda)
\stackrel{(c)}{\le} \inf_{\lambda \in \Lambda'} \sum_k \omega^{*k} \KL_k(\mu, \lambda)
\: .
\end{align*}
$(a)$ and $(b)$ are consequences of fact that $(\omega^*, q_{\omega^*})$ is a Nash equilibrium. $(c)$ comes from $\Lambda' \subseteq \Lambda$.

We proved that the value of an allocation $\omega^* \in \Omega(\Lambda)$ is at least as good as the value of any other allocation. Hence $\Omega(\Lambda) \subseteq \Omega(\Lambda')$.
\end{proof}

\begin{theorem}\label{thm:restricting_does_not_change_optimal_allocations}
Let $\varepsilon > 0$ and let $\Lambda_{\varepsilon} \subseteq \Lambda$ be such that for all $\lambda_\varepsilon \in \Lambda_{\varepsilon}$ and all $\omega \in \Omega(\Lambda)$, $\sum_{k = 1}^K \omega^k \KL_k(\mu, \lambda_\varepsilon) \ge \inf_{\lambda \in \Lambda} \sum_{k = 1}^K \omega^k \KL_k(\mu, \lambda) + \varepsilon$. Then $\Omega(\Lambda \setminus \Lambda_\varepsilon) = \Omega(\Lambda)$. 
\end{theorem}
\begin{proof}
We have the inclusion $\Omega(\Lambda) \subseteq \Omega(\Lambda \setminus \Lambda_\varepsilon)$ by Lemma~\ref{lem:optimal_alloc_restrict_alternative_subset}.

Now suppose that there exists $\omega' \in \Omega(\Lambda \setminus \Lambda_\varepsilon) \setminus \Omega(\Lambda)$. Let $\omega^* \in \Omega(\Lambda)$ be such that for all $r \in (0,1]$, $\omega_r := r \omega' + (1 - r) \omega^* \notin \Omega(\Lambda)$. We can get such an $\omega^*$ by taking an arbitrary $\omega^*_0 \in \Omega(\Lambda)$ and defining $\omega^* = r^* \omega' + (1 - r^*)\omega_0^*$, where $r^* = \sup \{r \in [0,1] \mid r \omega' + (1 - r)\omega_0^* \in \Omega(\Lambda)\}$. We know that $r^* < 1$ since $\Omega(\Lambda)$ is closed.

By convexity of $\Omega(\Lambda \setminus \Lambda_\varepsilon)$ and since both $\omega'$ and $\omega^*$ belong to that set, we have $\omega_r \in \Omega(\Lambda \setminus \Lambda_\varepsilon)$ for all $r \in [0,1]$.

Set $r \in (0,1]$. Since $\omega_r \notin \Omega(\Lambda)$, there exists $\lambda_r \in \Lambda$ such that $\sum_{k = 1}^K \omega_r^k \KL_k(\mu, \lambda_r) < \inf_{\lambda \in \Lambda} \sum_{k = 1}^K \omega^{*k} \KL_k(\mu, \lambda)$. It now suffices to show that for some $r \in (0,1]$, we have such a $\lambda_r$ with $\lambda_r \notin \Lambda_\varepsilon$. Indeed, under that condition we have that
\begin{align*}
\inf_{\lambda \in \Lambda \setminus \Lambda_\varepsilon} \sum_{k = 1}^K \omega_r^k \KL_k(\mu, \lambda)
\stackrel{(a)}{\le} \sum_{k = 1}^K \omega_r^k \KL_k(\mu, \lambda_r)
&\stackrel{(b)}{<} \inf_{\lambda \in \Lambda} \sum_{k = 1}^K \omega^{*k} \KL_k(\mu, \lambda)
\stackrel{(c)}{=} \inf_{\lambda \in \Lambda \setminus \Lambda_\varepsilon} \sum_{k = 1}^K \omega^{*k} \KL_k(\mu, \lambda)
\: .
\end{align*}
Inequality $(a)$ is due to the hypothesis $\lambda_r \in \Lambda \setminus \Lambda_\varepsilon$, $(b)$ is the definition of $\lambda_r$ and $(c)$ comes from the fact that minimizers over $\Lambda$ can't belong to $\Lambda_\varepsilon$ by definition of $\Lambda_\varepsilon$.
We then conclude that $\omega_r$ does not belong to $\Omega(\Lambda \setminus \Lambda_\varepsilon)$, which is a contradiction.

Let us now prove that there exists an $r \in (0,1]$ for which there exists $\lambda_r \in \Lambda \setminus \Lambda_\varepsilon$ with $\sum_{k = 1}^K \omega_r^k \KL_k(\mu, \lambda_r) < \inf_{\lambda \in \Lambda} \sum_{k = 1}^K \omega^{*k} \KL_k(\mu, \lambda)$.

If there is no such point, then since $\omega_r \notin \Omega(\Lambda)$ there exists $\lambda_{r,\varepsilon} \in \Lambda_\varepsilon$ such that $\sum_{k = 1}^K \omega_r^k \KL_k(\mu, \lambda_{r, \varepsilon}) < \inf_{\lambda \in \Lambda} \sum_{k = 1}^K \omega^{*k} \KL_k(\mu, \lambda)$.
But if $r$ is small enough we have
\begin{align*}
\inf_{\lambda \in \Lambda} \sum_{k = 1}^K \omega^{*k} \KL_k(\mu, \lambda)
> \sum_{k = 1}^K \omega_r^k \KL_k(\mu, \lambda_{r, \varepsilon})
&\ge (1 - r)\sum_{k = 1}^K \omega^{*k} \KL_k(\mu, \lambda_{r, \varepsilon})
\\
&\ge (1 - r)\left( \inf_{\lambda \in \Lambda} \sum_{k = 1}^K \omega^{*k} \KL_k(\mu, \lambda) + \varepsilon \right)
\\
&\ge \inf_{\lambda \in \Lambda} \sum_{k = 1}^K \omega^{*k} \KL_k(\mu, \lambda)
\: ,
\end{align*}
which is a contradiction.

\end{proof}

Remark: the hypothesis $\varepsilon > 0$ is necessary in Theorem~\ref{thm:restricting_does_not_change_optimal_allocations}. Indeed consider the unstructured Gaussian BAI problem in two dimensions in which $\mu = (0,2)$.
Then $\Lambda = \{\lambda \in \mathbb{R}^2 \mid \lambda_1 \ge \lambda_2 \}$ and the optimal allocation set is $\Omega(\Lambda) = \{(1/2, 1/2)\}$.
The only point with minimal value for that allocation is $\lambda_0 = (1,1)$.
Consider now $\Lambda_0 = \{\lambda_0\}$. Then $\Omega(\Lambda_0) = \triangle_2 \ne \Omega(\Lambda)$. In that restriction, we removed points arbitrarily close to the infimum value and Theorem~\ref{thm:restricting_does_not_change_optimal_allocations} does not apply.
